# Supplementary material for: Data-driven approach in a compartmental epidemic model to assess undocumented infections
Source: arXiv:2201.03476 ancillary file (2022-04-12)
Supplement: Supplementary file 1 [file suplementary.pdf]

# Supplementary Material:Data-driven approach in a compartmental epidemic model to assess undocumented infections

Guilherme S. Costa,[1] Wesley Cota,[1] and Silvio C. Ferreira[1,2]

[1] *Departamento de Física, Universidade Federal de Viçosa, 36570-900 Viçosa, Minas Gerais, Brazil*
[2] *National Institute of Science and Technology for Complex Systems, 22290-180, Rio de Janeiro, Brazil*

## I. SUPPLEMENTARY FIGURES

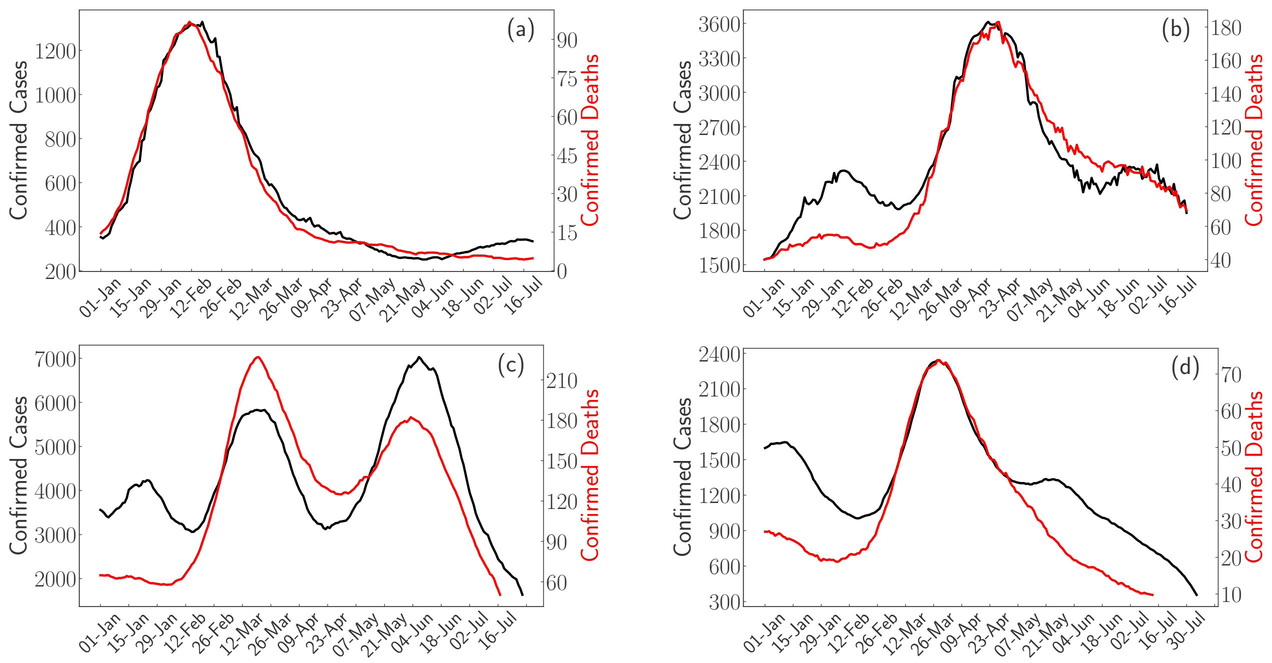


FIG. S1. Time series of confirmed cases (left axis, black curves) and deaths (right axis, red curves) for (a) Manaus/AM, (b) São Paulo/SP, (c) PR state and (d) ES state. Time series of death counts are shifted in (a) 7, (b) 9, (c) 10, and (d) 20 days, respectively.

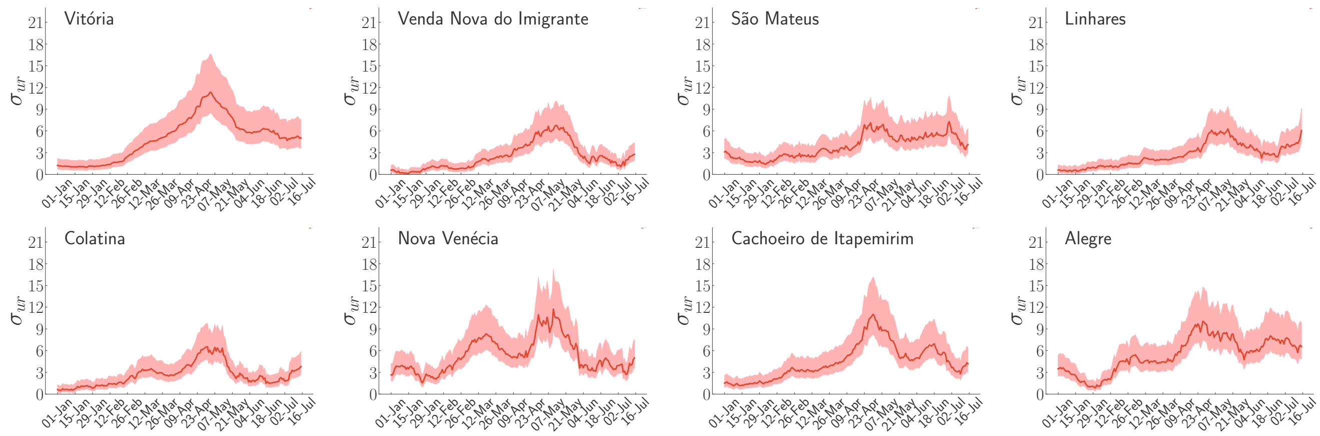


FIG. S2. Evolution of the under-reporting coefficient for immediate regions of ES state using time windows of 3 weeks. The regions are indicated in the upper-left corners for each panel.

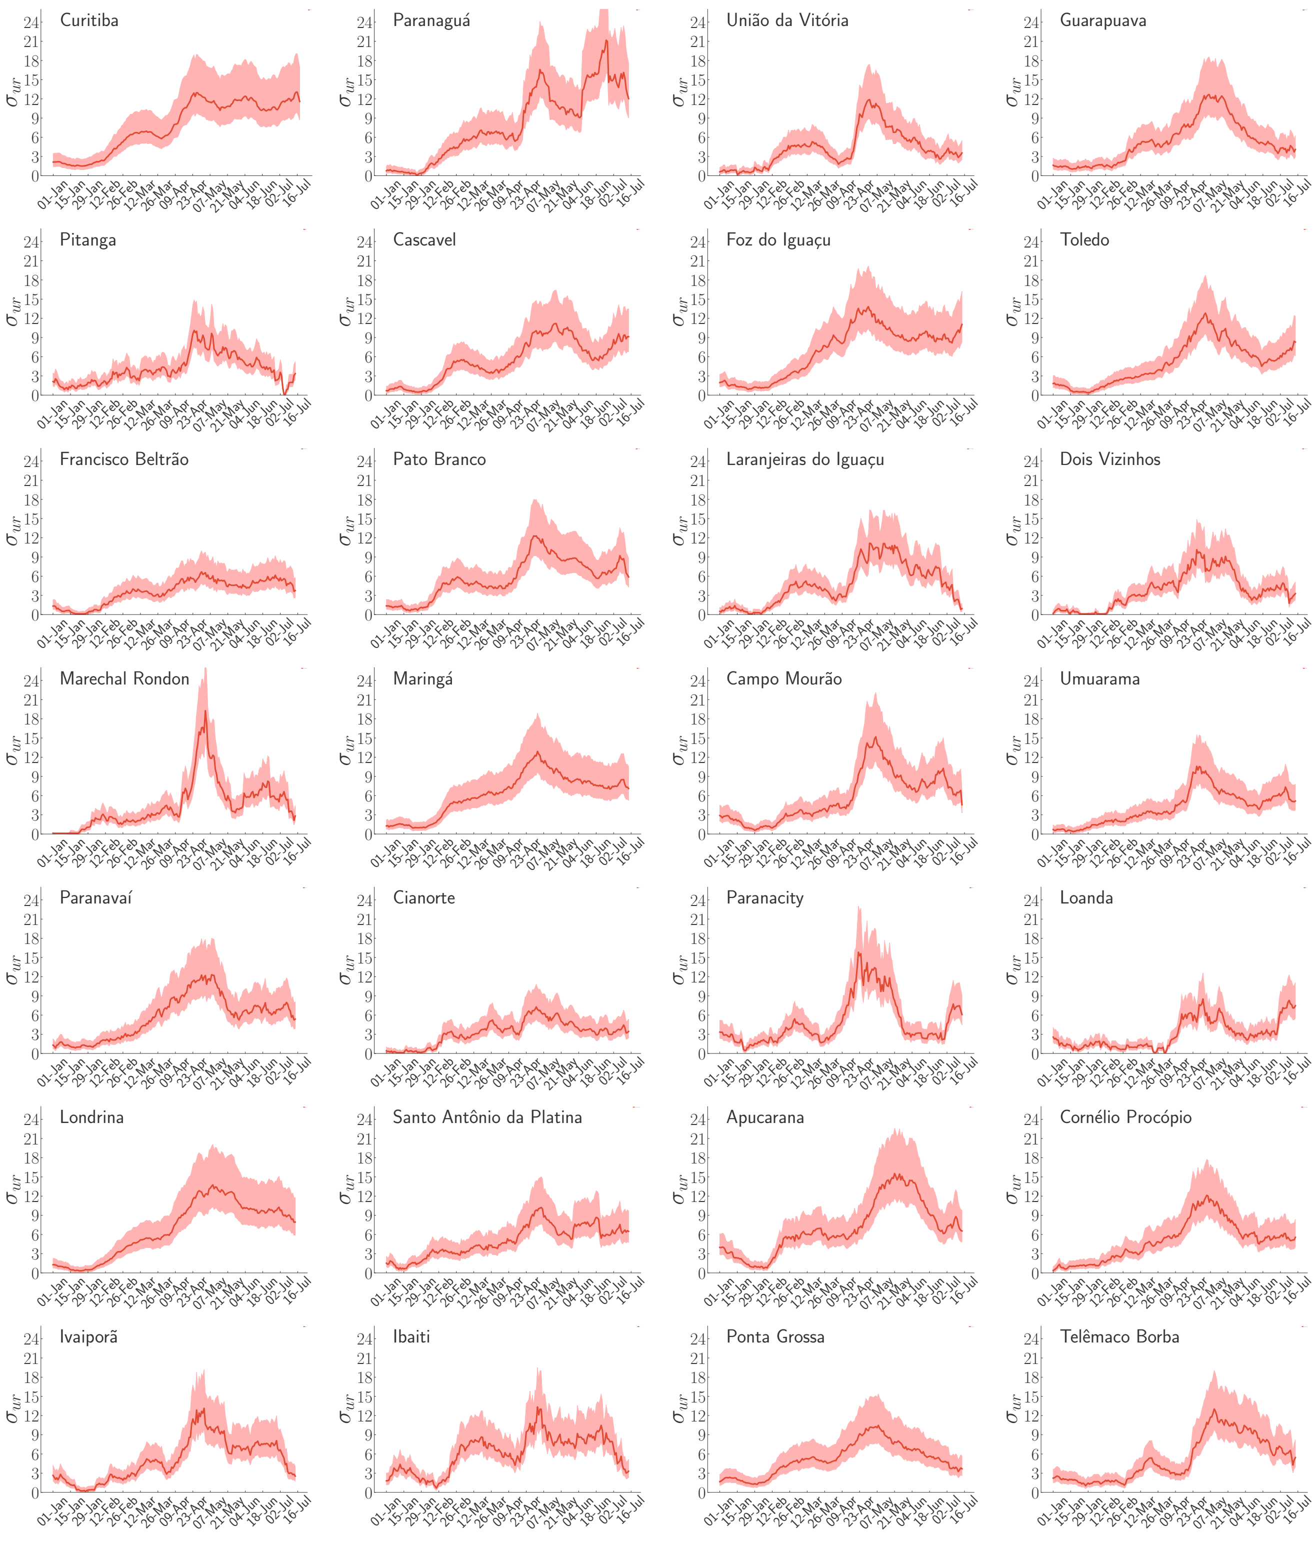


FIG. S3. Evolution of the under-reporting coefficient for immediate regions of PR state using time windows of 3 weeks. The regions are indicated in the upper-left corners for each panel.

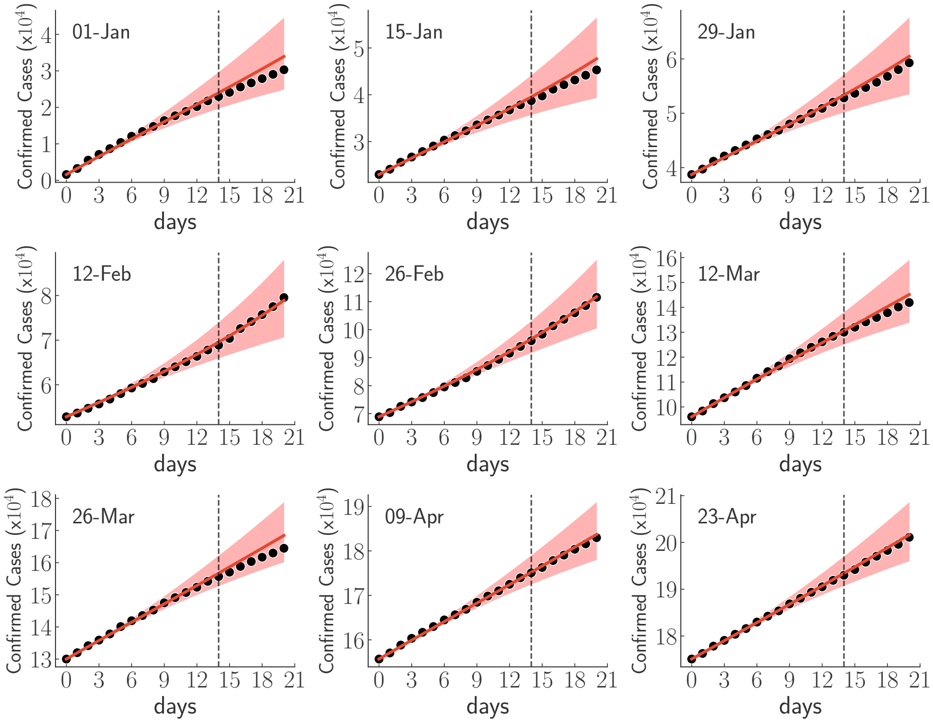


FIG. S4. Calibration curves for ES state in different time windows of 14 days indicated by the vertical lines. The initial day is indicated in the top of each panel. One week of forecasting is also shown. Symbols are the cumulative diagnosed cases while lines with shaded regions represent the calibrated curves and the corresponding confidence interval.

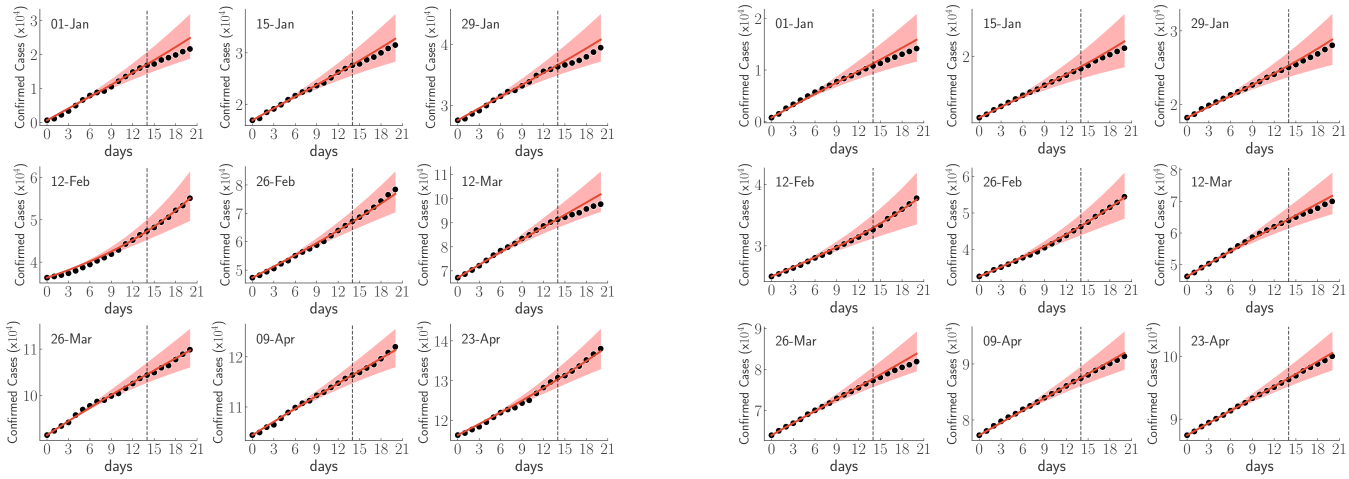


FIG. S5. Calibration curves for the immediate regions of (left panels) Curitiba and (right panels) Vitória in different time windows of 14 days indicated by the vertical lines. The initial day is indicated in the top of each panel. One week of forecasting is also shown. Symbols are the cumulative diagnosed cases while lines with shaded regions represent the calibrated curves and the corresponding confidence interval.

## II. DATA DESCRIPTION AND CODES

All data sets and codes used for calibration are publicly available at https://github.com/ghscosta/covid19-cal.

| Age group | IFR | Fraction of population | | | |
|---|---|---|---|---|---|
| | | PR | ES | AM | SP |
| 0-4 | 1.61e-05 | 0.0684 | 0.0707 | 0.0959 | 0.0656 |
| 5-9 | 1.61e-05 | 0.0668 | 0.0698 | 0.0967 | 0.0657 |
| 10-14 | 6.95e-05 | 0.0653 | 0.0672 | 0.0948 | 0.0638 |
| 15-19 | 6.95e-05 | 0.0701 | 0.0717 | 0.0922 | 0.0675 |
| 20-24 | 0.000309 | 0.0789 | 0.0773 | 0.0963 | 0.0744 |
| 25-29 | 0.000309 | 0.0800 | 0.0778 | 0.0879 | 0.0758 |
| 30-34 | 0.000844 | 0.0773 | 0.0831 | 0.0814 | 0.0823 |
| 35-39 | 0.000844 | 0.0757 | 0.0821 | 0.0765 | 0.0832 |
| 40-44 | 0.00161 | 0.0720 | 0.0751 | 0.0669 | 0.0766 |
| 45-49 | 0.00161 | 0.0672 | 0.0641 | 0.0542 | 0.0678 |
| 50-54 | 0.00595 | 0.0647 | 0.0599 | 0.0441 | 0.0627 |
| 55-59 | 0.00595 | 0.0582 | 0.0547 | 0.0352 | 0.0568 |
| 60-64 | 0.0193 | 0.0481 | 0.0467 | 0.0270 | 0.0489 |
| 65-69 | 0.0193 | 0.0381 | 0.0362 | 0.0195 | 0.0384 |
| 70-74 | 0.0428 | 0.0279 | 0.0245 | 0.0130 | 0.0280 |
| 75+ | 0.078 | 0.0405 | 0.0383 | 0.0177 | 0.0416 |

TABLE SI. Estimated infection fatality ratio of COVID-19 per age group and fraction of population of the feraderative states analyzed in the present work.

**Dictionary of municipalities:** The files (a) `dictES.csv` and (b) `dictPR.csv` of this supplementary material yield some information about municipalities of (a) ES (B) PR states. These files have six columns:

- `ID`: numeric key regarding calibration of confirmed cases time series
- `ibgeID`: official code to identify the city
- `name`: name of the city
- `intermID`: official code of intermediate region to which the city belongs
- `imedID`: official code of immediate region to which the city belongs
- `totPop2019`: population of the city estimated in 2019

**Dictionaries of immediate and intermediate regions:** The files (a) `dictImed.csv` and (b) `dictInterm.csv` of this supplementary material yield some information about (a) Immediate and (b) Intermediate regions. They were aggregated from `dictPR.csv` and `dictES.csv` files. These files have five columns:

- `ID`: numeric key regarding calibration of confirmed cases time series
- `imedID` or `intermID`: official code to identify the region
- `name`: name of the region
- `state`: state to which the region belongs
- `totPop2019`: population of the region estimated in 2019

**Dictionary of states:** The file `dictUF.csv` of this supplementary material yield some information about PR and ES states. They were aggregated from `dictPR.csv` and `dictES.csv` files. These files have five columns:

- `ID`: numeric key regarding calibration of confirmed cases time series

- `ibgeID`: official code to identify the state
- `name`: name of the state
- `uf`: abbreviation of the state's name
- `totPop2019`: population of the state estimated in 2019

**Time series of cases, deaths, and IFR:** The files (a) `PR.csv`, (b) `ES.csv`, (c) `saopaulo.csv`, and (d) `manaus.csv` of this supplementary material yield the time series of confirmed cases and deaths since January 1$^{\mathrm{st}}$, 2021 for (a) All cities of PR state, (b) All cities of ES state, (c) São Paulo city and (d) Manaus city. These files have eight columns:

- `date`: date
- `ibgeID`: official code to identify the city
- `newCases`: new confirmed cases on that day
- `newDeaths`: new confirmed deaths on that day
- `city`: name of the city
- `totalCases`: accumulated cases
- `totalDeaths`: accumulated deaths
- `ifr_vac`: infection fatality ratio due to vaccination

**Time series for calibration**: Within files (a) `imed.zip` and (b) `state.zip` we have the time series of accumulated cases and CFR, aggregated for different geographical scales. We provide two types of files: `casesXX.dat` are accumulated cases while `CFRXX.dat` are the daily CFRs (XX refers to the IBGE codes given in the dictionaries).

**Main code for calibration** : The file `calibra.f90` is a code in Fortran 90 that performs the calibration described in Methods' section of the main paper. A total of $i_{\mathrm{samp}} = 1, \ldots, 1000$ samples with epidemiological parameters drawn from their corresponding distributions are simulated. This code has four inputs: the time series of accumulated cases, CFR, initial date for calibration, and population of the region (state, city, etc). The code has two output files: `epiQuantities.dat` and `hiddenCompart.dat`. The first has seven columns: days from the initial time, calibrated confirmed cases, surveillance reported cases, $R_t$, fraction of susceptible population, $\sigma_{\mathrm{ur}}$, and sample label. The file `hiddenCompart.dat` yields time series for the following compartments from left to right: $S$, $E$, $A$, $I$, $C_{\mathrm{A}} + C_{\mathrm{I}}$, $R + R_{\mathrm{I}} + R_{\mathrm{A}} + D$, and sample label.
